# Supplementary material for: Probing Cross-modal Semantics Alignment Capability from the Textual Perspective
Source: arXiv:2210.09550 source file (2022-10-18)
Supplement: Supplementary file 1 [file tb_n_grams.tex]

% uniter
top ten 1-grams
[(('a',), 6192), (('the',), 4600), (('of',), 3892), (('room',), 382), (('people',), 366), (('cat',), 343), (('road',), 334), (('dog',), 331), (('apartment',), 328), (('playing',), 274)]
top ten 2-grams
[(('of', 'the'), 3487), (('a', 'man'), 273), (('a', 'group'), 265), (('a', 'young'), 249), (('holding', 'a'), 221), (('the', 'floor'), 210), (('the', 'downtown'), 207), (('skating', 'the'), 198), (('dog', 'dog'), 184), (('group', 'of'), 180)]
top ten 3-grams
[(('of', 'the', 'floor'), 207), (('a', 'group', 'of'), 180), (('of', 'the', 'downtown'), 173), (('the', 'floor', 'apartment'), 168), (('cat', 'of', 'the'), 166), (('a', 'cat', 'cat'), 164), (('cat', 'cat', 'of'), 162), (('group', 'of', 'people'), 157), (('bathroom', 'of', 'the'), 145), (('floor', 'apartment', 'apartment'), 142)]
top ten 4-grams
[(('of', 'the', 'floor', 'apartment'), 168), (('a', 'cat', 'cat', 'of'), 162), (('cat', 'cat', 'of', 'the'), 162), (('a', 'group', 'of', 'people'), 157), (('the', 'floor', 'apartment', 'apartment'), 142), (('a', 'bathroom', 'of', 'the'), 142), (('bathroom', 'of', 'the', 'floor'), 139), (('dog', 'dog', 'of', 'the'), 128), (('a', 'train', 'of', 'the'), 122), (('a', 'guy', 'skating', 'the'), 100)]

% rosita
top ten 1-grams
[(('a',), 39619), (('but',), 9613), (('that',), 5072), (('is',), 5066), (('image',), 4807), (('person',), 2500), (('man',), 1067), (('area',), 803), (('young',), 802), (('people',), 769)]
top ten 2-grams
[(('a', 'a'), 16611), (('but', 'a'), 8484), (('that', 'is'), 5066), (('is', 'a'), 5061), (('image', 'that'), 2945), (('a', 'image'), 2414), (('image', 'image'), 1820), (('a', 'person'), 1527), (('area', 'but'), 711), (('person', 'a'), 644)]
top ten 3-grams
[(('but', 'a', 'a'), 7173), (('that', 'is', 'a'), 5061), (('is', 'a', 'a'), 4981), (('image', 'that', 'is'), 2945), (('image', 'image', 'that'), 1820), (('a', 'image', 'image'), 1818), (('a', 'a', 'person'), 928), (('person', 'a', 'a'), 642), (('area', 'but', 'a'), 571), (('a', 'image', 'that'), 555)]
top ten 4-grams
[(('that', 'is', 'a', 'a'), 4981), (('image', 'that', 'is', 'a'), 2945), (('image', 'image', 'that', 'is'), 1820), (('a', 'image', 'image', 'that'), 1818), (('is', 'a', 'a', 'person'), 618), (('a', 'image', 'that', 'is'), 555), (('person', 'person', 'a', 'a'), 510), (('a', 'person', 'person', 'a'), 503), (('area', 'but', 'a', 'a'), 405), (('items', 'but', 'a', 'a'), 374)]

% vilbert
top ten 1-grams
[(('the',), 13881), (('at',), 10741), (('this',), 6877), (('a',), 6507), (('that',), 5631), (('was',), 3202), (('behind',), 2704), (('in',), 2652), (('towards',), 2616), (('some',), 1859)]
% [(('the',), 11474), (('at',), 10526), (('a',), 7353), (('this',), 5789), (('that',), 5642), (('towards',), 5173), (('some',), 3734), (('was',), 3009), (('inside',), 2774), (('beside',), 2340)]
top ten 2-grams
[(('at', 'this'), 5249), (('that', 'was'), 3009), (('at', 'some'), 2805), (('inside', 'the'), 2772), (('was', 'inside'), 2695), (('towards', 'the'), 2608), (('beside', 'the'), 1643), (('that', 'a'), 1567), (('towards', 'his'), 1184), (('that', 'the'), 996)]
top ten 3-grams
[(('that', 'was', 'inside'), 2695), (('was', 'inside', 'the'), 2695), (('at', 'this', 'person'), 644), (('at', 'this', 'party'), 595), (('party', 'at', 'some'), 564), (('this', 'person', 'at'), 541), (('this', 'party', 'at'), 516), (('a', 'man', 'that'), 502), (('at', 'this', 'restroom'), 484), (('this', 'restroom', 'beside'), 461)]
top ten 4-grams
[(('that', 'was', 'inside', 'the'), 2695), (('at', 'this', 'person', 'at'), 539), (('at', 'this', 'party', 'at'), 516), (('at', 'this', 'restroom', 'beside'), 461), (('this', 'restroom', 'beside', 'the'), 419), (('this', 'party', 'at', 'some'), 409), (('a', 'man', 'that', 'a'), 383), (('was', 'inside', 'the', 'sandwich'), 331), (('at', 'some', 'party', 'at'), 252), (('phone', 'that', 'was', 'inside'), 241)]

% clip 
top ten 1-grams
[(('a',), 24428), (('near',), 10031), (('area',), 6897), (('and',), 6252), (('image',), 6186), (('of',), 4320), (('background',), 3986), (('neck',), 1648), (('nearby',), 1435), (('player',), 1287)]
top ten 2-grams
[(('near', 'a'), 9910), (('and', 'a'), 4374), (('image', 'of'), 3999), (('area', 'and'), 3867), (('of', 'a'), 3490), (('a', 'image'), 2887), (('a', 'background'), 2482), (('image', 'image'), 2187), (('background', 'area'), 1211), (('player', 'player'), 975)]
top ten 3-grams
[(('image', 'of', 'a'), 3378), (('area', 'and', 'a'), 2676), (('near', 'a', 'background'), 2266), (('image', 'image', 'of'), 2187), (('a', 'image', 'image'), 1993), (('a', 'background', 'area'), 1193), (('a', 'image', 'of'), 894), (('player', 'player', 'player'), 669), (('a', 'background', 'top'), 618), (('top', 'nearby', 'background'), 572)]
top ten 4-grams
[(('image', 'image', 'of', 'a'), 2096), (('a', 'image', 'image', 'of'), 1993), (('near', 'a', 'background', 'area'), 1122), (('a', 'image', 'of', 'a'), 801), (('near', 'a', 'background', 'top'), 544), (('a', 'group', 'image', 'of'), 503), (('a', 'background', 'top', 'nearby'), 436), (('background', 'top', 'nearby', 'background'), 434), (('player', 'player', 'player', 'player'), 395), (('a', 'background', 'area', 'and'), 338)]

% lxmert
top ten 1-grams
[(('a',), 27242), (('of',), 12023), (('near',), 5216), (('sitting',), 1824), (('young',), 1783), (('tennis',), 1531), (('people',), 1471), (('standing',), 1427), (('holding',), 1139), (('posing',), 924)]
top ten 2-grams
[(('of', 'a'), 11458), (('near', 'a'), 4967), (('tennis', 'tennis'), 1201), (('holding', 'a'), 1099), (('wearing', 'a'), 805), (('on', 'a'), 761), (('a', 'young'), 758), (('young', 'young'), 720), (('posing', 'a'), 719), (('playing', 'a'), 657)]
top ten 3-grams
[(('tennis', 'tennis', 'tennis'), 1085), (('motorcycle', 'motorcycle', 'motorcycle'), 546), (('a', 'train', 'of'), 424), (('train', 'of', 'a'), 422), (('room', 'near', 'a'), 401), (('a', 'counter', 'near'), 399), (('counter', 'near', 'a'), 397), (('sitting', 'holding', 'a'), 390), (('of', 'a', 'train'), 375), (('a', 'young', 'young'), 355)]
top ten 4-grams
[(('tennis', 'tennis', 'tennis', 'tennis'), 970), (('motorcycle', 'motorcycle', 'motorcycle', 'motorcycle'), 476), (('a', 'train', 'of', 'a'), 405), (('a', 'counter', 'near', 'a'), 386), (('of', 'a', 'train', 'of'), 340), (('a', 'pizza', 'of', 'a'), 311), (('train', 'of', 'a', 'train'), 306), (('a', 'building', 'of', 'a'), 305), (('a', 'grass', 'near', 'a'), 285), (('a', 'room', 'near', 'a'), 282)]

% ce
top ten 1-grams
[(('a',), 12237), (('on',), 2298), (('of',), 2129), (('with',), 1865), (('in',), 1517), (('is',), 1307), (('and',), 1102), (('man',), 991), (('the',), 804), (('sitting',), 764)]
top ten 2-grams
[(('with', 'a'), 1701), (('on', 'a'), 1438), (('a', 'man'), 980), (('in', 'a'), 891), (('and', 'a'), 838), (('sitting', 'on'), 579), (('of', 'a'), 570), (('group', 'of'), 505), (('a', 'group'), 504), (('a', 'woman'), 470)]
top ten 3-grams
[(('a', 'group', 'of'), 504), (('sitting', 'on', 'a'), 427), (('group', 'of', 'people'), 331), (('a', 'man', 'is'), 313), (('on', 'top', 'of'), 276), (('next', 'to', 'a'), 269), (('a', 'man', 'riding'), 242), (('top', 'of', 'a'), 240), (('man', 'riding', 'a'), 233), (('in', 'a', 'field'), 232)]
top ten 4-grams
[(('a', 'group', 'of', 'people'), 331), (('on', 'top', 'of', 'a'), 240), (('a', 'man', 'riding', 'a'), 224), (('a', 'table', 'with', 'a'), 173), (('a', 'plate', 'of', 'food'), 147), (('a', 'bathroom', 'with', 'a'), 133), (('standing', 'in', 'a', 'field'), 133), (('in', 'front', 'of', 'a'), 128), (('group', 'of', 'people', 'standing'), 123), (('sitting', 'on', 'top', 'of'), 123)]
